# Supplementary material for: Thresholdless transition to coherent emission at telecom wavelengths from coaxial nanolasers
Source: arXiv:1905.09924 ancillary file (2019-05-23)
Supplement: Supplementary file 1 [file Kreinberg_et_al_SI.pdf]

# Thresholdless transition to coherent emission at telecom wavelengths from coaxial nanolasers

Sören Kreinberg,<sup>1</sup> Kaisa Laiho,<sup>1</sup> Frederik Lohof,<sup>2</sup> William Hayenga,<sup>3</sup> Paweł Holewa,<sup>1</sup>  
 Christopher Gies,<sup>2,\*</sup> Mercedeh Khajavikhan,<sup>3,†</sup> and Stephan Reitzenstein<sup>1,‡</sup>

<sup>1</sup>*Technische Universität Berlin, Institut für Festkörperphysik, Hardenbergstr. 36, 10623 Berlin, Germany*

<sup>2</sup>*Universität Bremen, Institut für Theoretische Physik, Otto-Hahn-Allee 1, 28359 Bremen, Germany*

<sup>3</sup>*CREOL, The College of Optics and Photonics, University of Central Florida, Orlando, FL, USA*

## S1. FABRICATION PROCEDURE AND SCANNING ELECTRON IMAGES

The fabrication steps involved in implementing metallic coaxial nanolasers (CNLs) are depicted below in Fig. S1. The wafer (grown by OEpic Inc.) consists of six quantum wells of  $\text{In}_{x=0.56}\text{Ga}_{1-x}\text{As}_{y=0.938}\text{P}_{1-y}$  (thickness: 10 nm), each sandwiched between two cladding layers of  $\text{In}_{x=0.734}\text{Ga}_{1-x}\text{As}_{y=0.57}\text{P}_{1-y}$  (thickness: 20 nm) with an overall height of 200 nm, grown on an InP substrate. The quantum wells are covered by a 10 nm thick InP over-layer for protection (Fig. S1a). An XR-1541 hydrogen silsesquioxane (HSQ) solution in methyl isobutyl ketone (MIBK) is used as a negative electron-beam resist. The resist is spun onto the wafer, resulting in a thickness of 100 nm (Fig. S1b). The nanolasers are then patterned by electron-beam lithography and are next immersed in tetramethylammonium hydroxide (TMAH) to develop the patterns (Fig. S1c). The electron beam alters the HSQ and turns it into a structure similar to  $\text{SiO}_2$ . The HSQ exposed to the electron beam now remains and serves as a mask for the subsequent reactive ion etching process. To perform the dry etching, a mixture of  $\text{H}_2$ :  $\text{CH}_4$ : Ar gas is used with a ratio of 40:6:15 sccm, RIE power of 150 W, and ICP power of 150 W at a chamber pressure of 35 mTorr (Fig. S1d). The wafer is then cleaned with

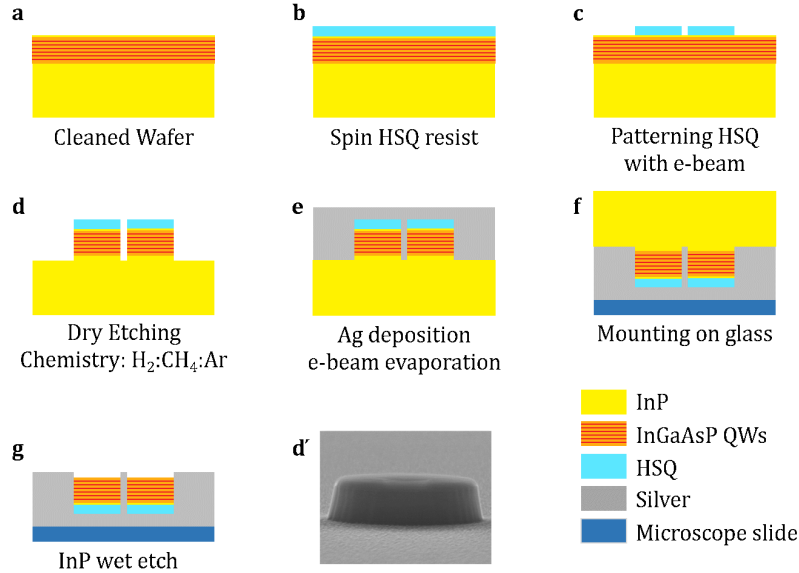

FIG. S1. Fabrication process of a coaxial nanolaser. The bottom right corner provides a legend to the materials of the structure. **a**, Cleaned wafer with InGaAsP Quantum wells grown on an InP substrate. **b**, A thin layer of negative tone HSQ ebeam resist is spun onto the sample. **c**, The wafer is patterned by electron beam lithography and the resist is developed. **d**, A dry etching process is used to define the cavity. **e**, 1  $\mu\text{m}$  Ag is deposited by means of electron-beam evaporation. **f**, The sample is mounted and bonded to a glass microscope slide silver side down with SU-8. **g**, The sample is immersed into HCl to remove the InP substrate. **d'**, Scanning electron microscope (SEM) image of a coaxial nanolaser after dry-etching, before the silver is deposited.

\* Corresponding author: gies@itp.uni-bremen.de

† Corresponding author: mercedeh@creol.ucf.edu

‡ Corresponding author: stephan.reitzenstein@physik.tu-berlin.de

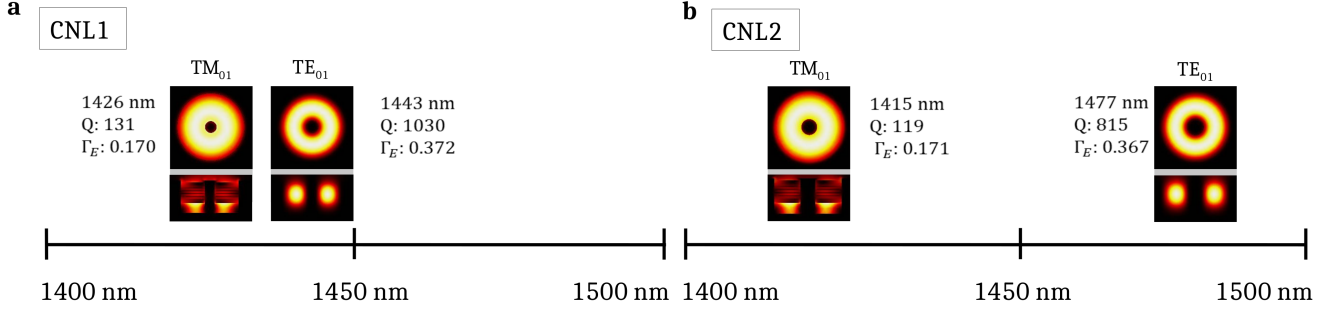

FIG. S2. A modal analysis of (a) CNL1 and (b) CNL2. The intensity profile of the modes between 1400 nm and 1500 nm are depicted on the plane of incident light (on top) and perpendicular to it (on bottom) together with the predicted wavelengths of the modes. A tolerance of 5 nm in the inner radii of the CNLs is accepted to match wavelengths of the lasing modes with the experiment. In both cases the lasing mode is the azimuthally polarized  $TE_{01}$ -like mode, which has the largest quality factor ( $Q$ ) and energy confinement ( $\Gamma_E$ ) by a relatively large margin marked in the figure.

oxygen plasma to remove organic contaminations and polymers that form during the dry etching process. After this, a 1000 nm layer of silver is deposited onto the sample using electron-beam evaporation at a pressure of  $5 \times 10^{-7}$  Torr at a rate of  $0.1 \text{ \AA s}^{-1}$  for the first 400 nm, at which point the rate is ramped up to  $1 \text{ \AA s}^{-1}$  (Fig. S1e). SU-8 is then used to bond the silver side to a glass substrate for support (Fig. S1f). Lastly, the sample is wet etched in hydrochloric acid to remove the InP substrate (Fig. S1g).

## S2. OPTICAL MODES

The eigenfrequencies of the cold cavity are found using finite element methods (COMSOL 3D Wave Optics Module). Both cavities have common dimensions of height (200 nm of InGaAsP quantum wells and barriers, 10 nm InP layer, 100 nm  $SiO_2$  plug, and 20 nm air plug). The six layers of quantum wells each having a height of 10 nm are embedded in seven barrier layers each having a height of 20 nm. CNL1 has an inner silver core radius of 55 nm and an outer radius of 295 nm, while CNL2 has an inner radius of 75 nm and outer radius of 315 nm, respectively. The relative permittivities used in the simulation are as follows at a temperature of 10 K: InGaAsP ( $\epsilon_g = 16.32$ ), barrier ( $\epsilon_b = 10.46$ ), InP ( $\epsilon_{InP} = 9.49$ ),  $SiO_2$  ( $\epsilon_{SiO_2} = 2.25$ ), and silver ( $\epsilon_{Ag} = -126 - i0.300$ ).

In addition to the TEM-like modes of these resonators [1], they are also capable of supporting modes similar to that observed in cylindrical metallic waveguides such as the azimuthally polarized  $TE_{01}$ -like mode, for example. The modal properties of the cavities are controlled by altering the inner and outer radii. Fig. S2(c-d) provide the modal analysis of CNL1 and CNL2 at a temperature of 10 K, respectively, that are found using COMSOL. In both cavities the  $TE_{01}$ -like mode has a much larger quality factor ( $Q$ ) and energy confinement factor ( $\Gamma_E$ ) than the other eigenfrequencies of the cavity and is the lasing mode. These figures of merit are given by  $Q = \frac{\omega}{2\kappa}$ , in which  $\omega$  is the angular frequency of the mode and  $2\kappa$  the cavity photon decay rate, and by  $\Gamma_E = \frac{\int_{V_a} d\mathbf{r} \epsilon(\mathbf{r}) |E(\mathbf{r})|^2}{\int_V d\mathbf{r} \epsilon(\mathbf{r}) |E(\mathbf{r})|^2}$ , in which  $V_a$  and  $V$  are the volume of the quantum wells and the total volume of the cavity, respectively,  $\epsilon$  is the relative permittivity of the different layers and  $E(\mathbf{r})$  the simulated electric field in terms of the spatial position  $\mathbf{r}$ . In CNL1 the  $TM_{01}$ -like and  $TE_{01}$ -like modes are both near the peak of the gain. In CNL2 the size of the cavity is increased, in turn shifting the resonance of the  $TE_{01}$ -like mode to a higher wavelength, far away from the maximum gain, which in turn results in a lower effective  $\beta$ -factor.

## S3. EXPERIMENTAL SETUP

For our optical and quantum optical investigations we use the experimental setup as shown in Fig. S3. A linearly polarized continuous-wave (CW) external cavity diode laser with emission at 980 nm is used to optically excite the CNL under study. We employ a confocal excitation and detection scheme, in which the CW laser is focused on the sample placed in a He-flow cryostat at 10 K with a microscope objective having a focal length of 10 mm and a numerical aperture of 0.4. The objective is mounted on a three-axis piezo stage for precise adjustment of the excitation spot with sub-micrometer accuracy. The light emitted from the CNL is collected and collimated with the same objective and then separated from the excitation laser with a cold mirror. A long-pass filter with the cut-on edge at  $1 \mu\text{m}$  is

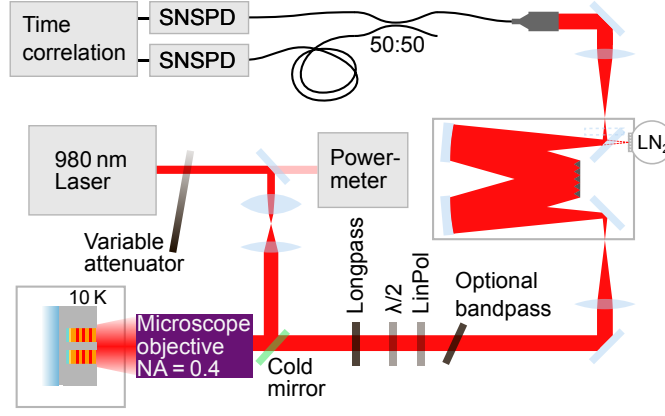

FIG. S3. Experimental arrangement. A variably attenuated 980 nm excitation laser is sent to the CNLs residing at 10 K. After separating the CNL emission from pump light, its spectrum and polarization is controlled with bulk optics. The emission spectra are acquired with a grating spectrograph using a liquid nitrogen (LN<sub>2</sub>) cooled InGaAs array. For the HBT-measurements the spectrograph is used in transmission and the light is launched via a fibre-coupled symmetric beams splitter at two SNSPDs for time-dependent coincidence discrimination.

used for suppressing residual background light before the emitted light is sent via a half-wave plate ( $\lambda/2$ ), a linear sheet polarizer (LinPol) and an optional tunable bandpass filter to a Czerny-Turner spectrograph with focal length of 750 mm. For the spectral measurements we use gratings with 150 lines/mm and 900 lines/mm leading to spectral resolutions of 0.33 and 0.05 nm, respectively. Thereafter, either a 1D InGaAs array is used for detecting the spectra of the emitted light or the light is coupled out of the spectrograph via its exit-slit and directed to a single-mode 50:50 fiber-splitter for an HBT measurement, which is equipped with two superconducting nanowire single photon detectors (SNSPDs) with a specified dark count rate of  $\leq 10 \text{ s}^{-1}$  and a timing jitter of  $\leq 50 \text{ ps}$ . A fiber optical delay is used to avoid the detector cross-talk by shifting the physical zero-time-delay away from the detector zero-time-delay.

For the broadband HBT measurement, we set the grating angle to zero order such that it acts like a normal mirror and the monochromator thus transmits the beam of light without spectral resolution. In this configuration the laser mode is selected by the 12 nm broad, almost a brick-wall shaped bandpass filter. For the spectrally narrowband HBT measurements, we perform a second series of excitation intensity-dependent measurements of  $g^{(2)}(\tau)$  for CNL1, this time using the  $900 \text{ mm}^{-1}$  grating in first refractive order. Thus, the location of the laser spot on the fiber facet depends on the wavelength, resulting in spectral filtering with an estimated FWHM of 22 pm. This estimate is calculated as follows: We assume the modes from the nanolaser at the monochromator exit slit to be Gaussian. We also make this assumption for the mode of the fiber. We then calculate the mode overlap  $\eta$  of the nanolaser mode  $E_n$  and the fiber mode  $E_f$  at the position  $r$  of the monochromator exit slit, if the nanolaser mode is shifted sideways by distance  $d$ :

$$E_n(r) = \exp\left(-\frac{(r-d)^2}{m_n^2}\right)$$

$$E_f(r) = \exp\left(-\frac{(r)^2}{m_f^2}\right)$$

$$\eta(d) = \frac{\left|\int_{-\infty}^{\infty} E_n(r) E_f^*(r) dr\right|^2}{\int_{-\infty}^{\infty} |E_n(r)| dr \int_{-\infty}^{\infty} |E_f(r)| dr}$$

Note, that  $m_n$  and  $m_f$  correspond to the mode field radius of the respective Gaussian mode. We then calculate the FWHM  $\Delta d$  of the mode overlap  $\eta$  with respect to the lateral displacement  $d$  by solving

$$\eta(\Delta d) = \frac{\eta(d=0)}{2},$$

resulting in

$$\Delta d = \sqrt{m_n^2 + m_f^2} \sqrt{\ln 4}.$$

We introduce a parameter  $k = m_n/m_f$ , which corresponds to the matching of the mode field diameters. Using our knowledge of the fiber mode field diameter  $MFD_f = 10 \mu\text{m}$ , the focal length of the lens behind the monochromator

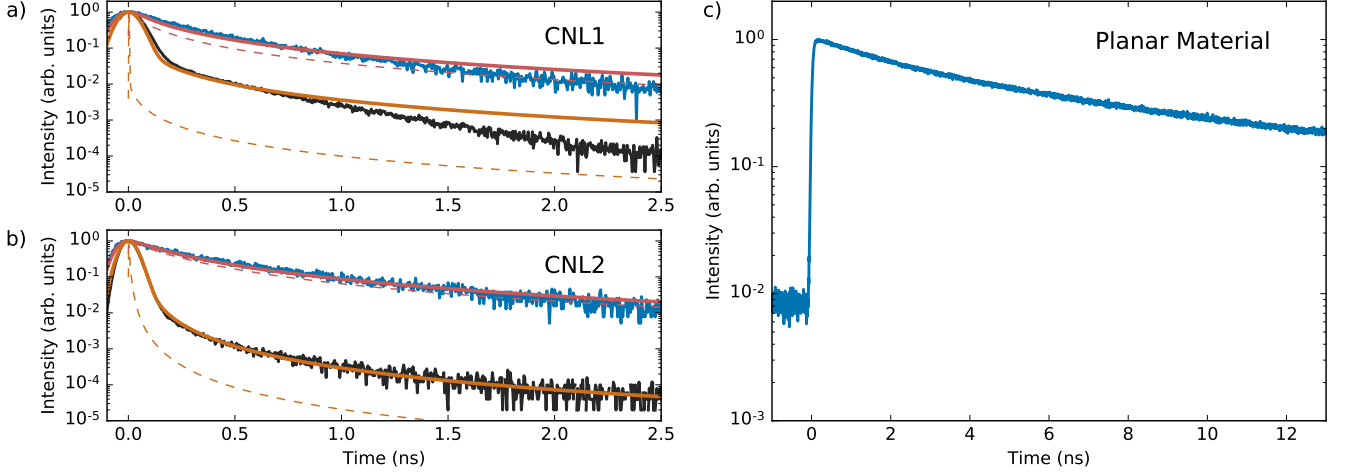

FIG. S4. Luminescence time traces for **a)** CNL1, **b)** CNL2 and **c)** the planar laterally non-confined gain material. For measuring the spontaneous emission lifetime, low energy excitation pulse of approximately 40 fJ (blue curves) where chosen, while stronger pulses of 2 pJ (black curves) where used to demonstrate lasing. Theoretical calculation of cavity luminescence (red/orange) allows to choose an appropriate rate of light-matter interaction. Calculated traces (dashed lines) are convoluted with the response function of the detector used in the measurement in order to reach good agreement (solid lines). Lifetime measurement on the planar gain material, suggest strongly enhanced spontaneous emission. Although the decay does not follow an exponential law, the planar materials luminescence decays on time scales of  $\sim 6$  ns, while the CNLs' lifetimes are  $< 0.4$  ns indicating a pronounced Purcell effect, mediated by the metal cavities. The spike at the beginning of the each black curves is attributed to stimulated emission and cannot be resolved with the SNSPDs. It gives however, striking proof of lasing action.

$f_{\text{mono}} = 40$  mm and the lens in front of the fiber (included in the fiber collimator)  $f_{\text{coll}} = 15.29$  mm, the dispersion per pixel  $\delta\lambda_{\text{px}} = 25$  pm and the pixel size  $s_{\text{px}} = 25$   $\mu\text{m}$  to calculate the FWHM  $\Delta\nu$  of the spectral acceptance of the fiber via

$$m_f = \frac{1}{2} \frac{f_{\text{mono}}}{f_{\text{coll}}} MFD_f$$

$$\Delta\nu = \frac{\delta\lambda_{\text{px}}}{s_{\text{px}}} \Delta d$$

to

$$\Delta\nu = 21.8 \text{ pm},$$

if a value of  $k = 1$  is chosen.  $k = 1$  is a legitimate assumption, because the lenses in the setup were especially chosen such that a fully illuminated microscope objective fills the monochromator grating without being cropped and that the monochromator grating dimension is matched to the numerical aperture of the fiber mode.

#### S4. LIFETIME MEASUREMENT

A considerable Purcell enhancement of the radiative decay rate is expected to be observed due to strong optical confinement in the CNLs. In order to investigate this parameter, we excite the gain material with 40 fJ picosecond optical pulses (weak enough to stay below the lasing threshold) and measure the excitation lifetime inside the CNLs and compare it to a flake of planar gain material (i.e. w/o optical cavity). The lifetime measurement is implemented as a start-stop time correlation experiment with the pump laser pulses triggering the start and photons from the CNLs triggering the stop. For excitation we use a Ti:sapphire laser with a central wavelength of 770 nm and a repetition rate of 80 MHz. Optionally, the pump laser can be sent through an acousto-optical modulator (AOM), which only deflects every 8th pulse towards the excitation fiber, reducing the repetition rate to 10 MHz and thus achieving a free 100 ns window for the lifetime measurements. The electrical trigger from the laser/AOM is sent to the time correlator as the start signal. The pulsed/pulse-picked excitation laser is coupled into the experimental setup similarly to the 980 nm laser as shown in Fig. S3. The emission from the CNLs and from the planar gain material is spectrally

selected by the 12 nm broad bandpass filter, spectrally centered around the CNLs lasing wavelengths and is detected by a single SNSPD. Signals from this SNSPD mark the stop time of the time correlator. The histograms for the start-stop measurement with (CNLs) and without the cavity (i.e. obtained from planar gain material) are shown in Fig. S4 (blue curves) while additional evidence of lasing is also gained from the lifetime measurement by using stronger excitation pulses (2 pJ) for driving the CNLs into the regime of stimulated emission (black curves).

Looking at the time traces, it is clear that the measurements cannot be modeled by simple exponential decays. Instead we employ our quantum optical model to calculate the Purcell-enhanced spontaneous emission from the cavity and obtain good agreement with experimental results for both CNLs (red/orange curves, see Sec. S5 for further details). We clearly see that the planar gain material has a much longer lifetime on the order of 6 ns than the gain material confined in the CNL cavities, where luminescence decays on a time scale of  $< 0.4$  ns. The lifetime ratios of the radiative decay processes suggests a strong Purcell enhancement factor of approximately 15. As we point out in the section “Modeling of CNL luminescence” in Sec. S5, matching the theoretical calculation to the measured data is important to confirm the value of the light-matter coupling strength in the quantum-optical modeling.

## S5. QUANTUM THEORY OF CNL EMISSION

We use a quantum optical semiconductor laser theory to calculate the input-output characteristics, the zero-delay time second-order photon-correlation function  $g^{(2)}(\tau = 0)$ , the coherence time, and the linewidth. The latter two are obtained from a two-time calculation of the first-order autocorrelation function  $g^{(1)}(t, \tau)$ . In effective-mass approximation, we consider a quasi continuum of  $k$  states with electron momentum  $\hbar k$ , where  $\hbar$  is the reduced Planck constant. QW carriers interact with the TE<sub>01</sub>-like mode of the CNL cavity. By quantizing the light field we access the statistical properties of the emitted photons via the autocorrelation functions  $g^{(2)}(\tau = 0)$  and  $g^{(1)}(\tau)$ . In the following,  $b^\dagger$  and  $b$  denote creation and annihilation operators for photons in the cavity mode, while operators  $c_k$  and  $v_k$  refer to electrons in the conduction and valence band of the semiconductor gain material. The system Hamiltonian is given by

$$H = H_{\text{carr}} + H_{\text{ph}} + H_I, \quad (\text{S1})$$

with

$$H_{\text{carr}} = \sum_k \epsilon_k^e c_k^\dagger c_k + \sum_k \epsilon_k^h v_k^\dagger v_k, \quad (\text{S2})$$

$$H_{\text{ph}} = \hbar\omega \left( b^\dagger b + \frac{1}{2} \right), \quad (\text{S3})$$

$$H_I = i \sum_k \left( g_k b v_k c_k^\dagger - g_k^* b^\dagger v_k^\dagger c_k \right), \quad (\text{S4})$$

where  $H_{\text{carr}}$  and  $H_{\text{ph}}$  are the Hamiltonians of the charge carriers and photons, and  $H_I$  is the light-matter interaction Hamiltonian. The energies  $\epsilon_k^e$  and  $\epsilon_k^h$  are the energies of single electrons and holes and  $\hbar\omega$  is the cavity mode energy. The light-matter interaction strength  $g_k$  for an homogeneous quantum well interacting with a the localized mode of a cavity we define as

$$g_k = \sum_{\mathbf{q}_{\parallel}} 2E_{\text{ph}} \Gamma_z \mathbf{d}_k \cdot \tilde{\mathbf{u}}(\mathbf{q}_{\parallel}), \quad (\text{S5})$$

with  $E_{\text{ph}} = \sqrt{\frac{\hbar\omega}{2\epsilon_0 V_m}}$  the field per photon,  $V_m$  the mode volume,  $\Gamma_z$  the geometrical confinement factor (vertical to the QW) and  $\tilde{\mathbf{u}}(\mathbf{q}_{\parallel})$  the Fourier transform of the (cavity-) mode function inside the QW plane. The dipole moment for the transition from the conduction to the valence band can be expressed as [2]

$$\mathbf{d}_k = \frac{\mathbf{d}_0}{1 + \frac{\hbar^2 k^2}{2m_r \epsilon_g}}, \quad (\text{S6})$$

where  $\mathbf{d}_0$  is the dipole moment at  $k = 0$ ,  $m_r$  is the reduced mass of the applied two band model and  $\epsilon_g$  is the band-gap energy of the material at zero excitation.

### Coupled laser equations

From the system Hamiltonian and using Heisenberg's equation of motion for expectation values we derive dynamical equations for the average photon number  $\langle b^\dagger b \rangle$  in the cavity and population functions of electrons  $f_k^e = \langle c_k^\dagger c_k \rangle$  and holes  $f_k^h = 1 - \langle v_k^\dagger v_k \rangle$  in conduction and valence bands:

$$\left( \frac{d}{dt} + 2\kappa \right) \langle b^\dagger b \rangle = 2 \sum_k |g_k|^2 \text{Re} \left[ \langle b^\dagger v_k^\dagger c_k \rangle \right], \quad (\text{S7})$$

$$\frac{d}{dt} f_k^e = -2|g_k|^2 \text{Re} \left[ \langle b^\dagger v_k^\dagger c_k \rangle \right] - \gamma_{\text{nl}} f_k^e f_k^h - \gamma_{\text{rel}} (f_k^e - f_k^{\text{F.D.}}) + P f_k^{(0)} (1 - f_k^e), \quad (\text{S8})$$

$$\frac{d}{dt} f_k^h = -2|g_k|^2 \text{Re} \left[ \langle b^\dagger v_k^\dagger c_k \rangle \right] - \gamma_{\text{nl}} f_k^e f_k^h - \gamma_{\text{rel}} (f_k^h - f_k^{\text{F.D.}}) + P f_k^{(0)} (1 - f_k^h), \quad (\text{S9})$$

with rates of radiative losses  $\gamma_{\text{nl}}$ , and carrier relaxation  $\gamma_{\text{rel}}$  as well as pump rate  $P$  (see below). In the derivation we employed the cluster expansion technique as a consistent truncation scheme for the arising hierarchy of coupled equations [3]. The coherent light-matter interaction is mediated by the photon-assisted polarization  $\langle b^\dagger v_k^\dagger c_k \rangle$ , associated with a carrier transition from a conduction-band to a valence-band state  $k$  under creation (emission) of a photon. Other processes are included by Lindblad terms or on a phenomenological basis. The photon losses are accounted for by the cavity decay rate  $2\kappa = \omega/Q$ , while the carrier-population functions are subject to radiative losses as well as pumping.

We consider an external pump process for excitation of carriers in the barrier at a rate  $P$  followed by subsequent capture in the QWs' quasi-continuum states. This is modeled by Gaussian carrier generation ( $f_k^{(0)}$ ) sufficiently high above the band gap (2.2 eV) such that no optically active states are pumped. Pauli blocking is accounted for by the factor  $1 - f_k^{e/h}$ . We use the relaxation time approximation with rate  $\gamma_{\text{rel}}$  that relaxes carriers into quasi equilibrium  $f_k^{\text{F.D.}}$  separately for conduction and valence bands.

Radiative losses into non lasing modes are typically associated with the  $\beta$ -factor, which is defined as the fraction of spontaneous emission that is directed into the lasing mode. It is also related to the occurrence of a threshold jump in the input-output characteristic and the "steepness" of the lasing transition, i.e. for  $\beta$ -factors close to unity the transition to coherent emission is more gradual. For radiative losses to occur the presence of both, an electron and hole is required, thus the dependence on the product  $f_k^e f_k^h$ . Furthermore the rate of radiative recombination is generally  $k$ -dependent and depends on the change of the photonic density of states mediated by the surrounding cavity. However, as recombination is typically much slower than redistribution of carriers due to relaxation, we treat the process with one effective  $k$ -independent recombination rate  $\gamma_{\text{nl}}$ . Generally, non radiative-loss processes can be included as well [4] but we refrain from including them here as we consider them negligible in the present case.

The equation of motion for the photon assisted polarization  $\langle b^\dagger v_k^\dagger c_k \rangle$  contains the central processes that arise from the light-matter interaction

$$\begin{aligned} \left( \frac{d}{dt} + \kappa + \Gamma \right) \langle b^\dagger v_k^\dagger c_k \rangle &= -i(\epsilon_k^e - \epsilon_k^h - \hbar\omega) \langle b^\dagger v_k^\dagger c_k \rangle \\ &\quad + f_k^e f_k^h + \langle b^\dagger b \rangle (f_k^e + f_k^h - 1) \\ &\quad + \delta \langle b^\dagger b c_k^\dagger c_k \rangle - \delta \langle b^\dagger b v_k^\dagger v_k \rangle. \end{aligned} \quad (\text{S10})$$

The free evolution is determined by the individual detuning between the carrier transitions  $\epsilon_k^e - \epsilon_k^h$  and the central cavity mode energy  $\hbar\omega$ . The quantum-optical treatment of the light field gives rise to a spontaneous emission term  $f_k^e f_k^h$  and stimulated processes given by  $\langle b^\dagger b \rangle (f_k^e + f_k^h - 1)$  are proportional to the photon number as well as the carrier inversion which, depending on the sign of the population functions represent gain or absorption of the material. The bandwidth of the interaction is determined by the broadening of the cavity resonance  $\kappa$  and that of the optical transitions in the material, which we model with a constant dephasing rate  $\Gamma$  [2].

The carrier-photon correlation functions  $\delta\langle b^\dagger b c_k^\dagger c_k \rangle$  and  $\delta\langle b^\dagger b v_k^\dagger v_k \rangle$  go beyond the treatment that is encountered in the derivation of laser rate equations. While generally they present only a minor correction to the quantities in Eqs. (S7)–(S9) [5], their inclusion is central to the calculation of the second-order correlation function given by

$$g^{(2)}(\tau = 0) = 2 + \frac{\delta\langle b^\dagger b^\dagger b b \rangle}{\langle b^\dagger b \rangle^2}, \quad (\text{S11})$$

for which four additional equations are required

$$\left(\frac{d}{dt} + 4\kappa\right) \delta\langle b^\dagger b^\dagger b b \rangle = 4 \sum_{k'} |g_{k'}|^2 \text{Re} \left[ \delta\langle b^\dagger b^\dagger b v_{k'}^\dagger c_{k'} \rangle \right], \quad (\text{S12})$$

$$\begin{aligned} \left(\frac{d}{dt} + 3\kappa + \Gamma\right) \delta\langle b^\dagger b^\dagger b v_k^\dagger c_k \rangle = & -i(\epsilon_k^e - \epsilon_k^h - \hbar\omega_l) \delta\langle b^\dagger b^\dagger b v_k^\dagger c_k \rangle \\ & - 2|g_k|^2 \langle b^\dagger v_k^\dagger c_k \rangle^2 - (1 - f_k^e - f_k^h) \delta\langle b^\dagger b^\dagger b b \rangle \\ & + 2f_k^h \delta\langle b^\dagger b c_k^\dagger c_k \rangle - 2f_k^e \delta\langle b^\dagger b v_k^\dagger v_k \rangle \\ & + 2\langle b^\dagger b \rangle (\delta\langle b^\dagger b c_k^\dagger c_k \rangle - \delta\langle b^\dagger b v_k^\dagger v_k \rangle), \end{aligned} \quad (\text{S13})$$

$$\left(\frac{d}{dt} + 2\kappa\right) \delta\langle b^\dagger b c_k^\dagger c_k \rangle = -2|g_k|^2 \text{Re} \left[ \delta\langle b^\dagger b^\dagger b v_k^\dagger c_k \rangle + (\langle b^\dagger b \rangle + f_k^e) \langle b^\dagger v_k^\dagger c_k \rangle \right], \quad (\text{S14})$$

$$\left(\frac{d}{dt} + 2\kappa\right) \delta\langle b^\dagger b v_k^\dagger v_k \rangle = 2|g_k|^2 \text{Re} \left[ \delta\langle b^\dagger b^\dagger b v_k^\dagger c_k \rangle + (\langle b^\dagger b \rangle + f_k^h) \langle b^\dagger v_k^\dagger c_k \rangle \right]. \quad (\text{S15})$$

The closed system of equations (S7)–(S15) is obtained by neglecting higher order correlations along the lines of [3]. For numerical evaluation we apply the Markov approximation, which is exact in the steady state. In order to do so we solve Eqs. (S10) and (S13) adiabatically and substitute them in all other equations. This approach is straight-forward since we assume a constant dephasing rate for all  $k$ -stats. However, the resulting Lorentzian linewidth functions overestimate the bandwidth of the interaction resonance due to slowly decreasing tails. To amend this, we substitute the Lorentz linewidth function according to [2]

$$L(k) = \frac{\xi^2}{\xi^2 + (\epsilon_k - \hbar\omega)^2} \rightarrow \text{sech}\left(\frac{\epsilon_k - \hbar\omega}{\xi}\right), \quad (\text{S16})$$

where  $\epsilon_k - \hbar\omega$  denotes the detuning between the electronic transitions and the cavity mode energy, and  $\xi$  the width of the corresponding lineshape. Note that substitution of the lineshape function does not change the total strength of the interaction as the area under the curves is preserved.

### Coherence time and emission linewidth

The coherence time and linewidth of the emission are related to the two-time first-order correlation function

$$g^{(1)}(t, \tau) = \frac{\langle b^\dagger(t) b(t + \tau) \rangle}{\langle b^\dagger(t) b(t) \rangle}.$$

Its dynamics can be obtained from the Heisenberg equation of motion, taking the first argument to correspond to the steady-state time, and the time derivative is taken with respect to the delay time  $\tau$ :

$$\frac{d}{d\tau} G(\tau) = \sum_k g_k^* P_k(\tau) - (\kappa + i\hbar\omega) G(\tau), \quad (\text{S17})$$

$$\frac{d}{d\tau} P_k(\tau) = g_k (f_k^c - f_k^v) G(\tau) - (\Gamma + i(\epsilon_k^e - \epsilon_k^h)) P_k(\tau). \quad (\text{S18})$$

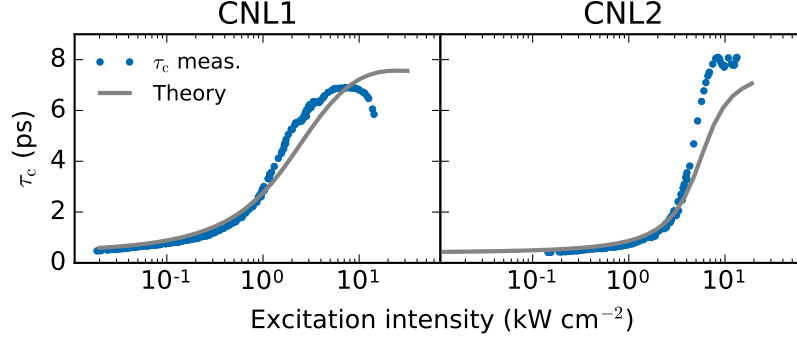

FIG. S5. Coherence time  $\tau_c$  as function of excitation intensity. Measured values are estimated from linewidths given in Fig. 3 (g-h) in the main text. Theoretical values are obtained from Eq. (S21). Both, experiment and theory, show an saturation of the coherence time at moderate coherence times  $\tau_c < 8$  ps.

with the abbreviations

$$G(\tau) = \langle b^\dagger(t)b(t+\tau) \rangle, \quad (\text{S19})$$

$$P_k(\tau) = \langle b^\dagger(t)v_k^\dagger(t+\tau)c_k(t+\tau) \rangle. \quad (\text{S20})$$

Initial conditions for Eqs. (S17) and (S18) are given by  $G(0) = \langle b^\dagger b \rangle$  and  $P_k(0) = \langle b^\dagger v_k^\dagger c_k \rangle$ . Together with stationary populations of conduction and valence bands  $f_k^c$  and  $f_k^v$ , they are obtained from stationary solutions of the dynamic laser equations (S7)–(S15) [6].

The coherence time is given by

$$\tau_c = \int_{-\infty}^{\infty} d\tau \left| g^{(1)}(t, \tau) \right|^2, \quad (\text{S21})$$

and the linewidth is read off as the FWHM of the normalized power spectral density defined as [7]

$$\mathcal{F}(\omega) = \frac{1}{\pi} \text{Re} \int_0^{\infty} d\tau g^{(1)}(\tau) e^{i\omega\tau}. \quad (\text{S22})$$

While for the measured  $g^{(2)}(0)$  was deconvoluted, taking into account an estimate for the coherence time (see Methods in the main text), the theoretical calculation proceeds in the opposite direction. We also assume the Siegert relation  $g^{(2)}(\tau) = 1 + a|g^{(1)}(\tau)|^2$ , where the calculated result from Eq. (S11) enters via  $a = g^{(2)}(0) - 1$  [7]. In a second step the time dependent  $g^{(2)}(\tau)$  is convoluted with the detector response function, assumed to be a Gaussian with  $\sigma = \Delta t / (2\sqrt{2\ln(2)})$  and FWHM  $\Delta t = 80$  ps, in order to model the measured  $\tilde{g}^{(2)}(\tau)$ . As we only plot the value at  $\tau = 0$  we specifically calculate

$$\tilde{g}^{(2)}(0) = 1 + (g^{(2)}(0) - 1) \int_{-\infty}^{\infty} d\tau |g^{(1)}(\tau)|^2 \frac{1}{\sqrt{2\pi\sigma^2}} e^{-\frac{\tau^2}{2\sigma^2}}. \quad (\text{S23})$$

Theoretically predicted coherence times that enter the calculation of  $\tilde{g}^{(2)}(0)$  are shown in Fig. S5 together with experimental values estimated from linewidth measurements of the CNLs emission (see Fig. 3g,h in the main text).

### Modeling of CNL luminescence

The introduced laser model allows for the calculation of time-resolved photoluminescence (TRPL) of the CNLs following excitation. We do so by integrating Eqs. (S7)–(S10) over time while neglecting the higher order correlations

in the last line in Eq. (S10). We assume instantaneous carrier generation by a laser pulse and start the calculation at a fixed carrier density. Calculated normalized TRPL traces are shown in Fig. S4 (dashed lines) for both CNLs at high and low excitation, choosing initial densities well below (red) and well above (orange) the threshold region in the steady state results. The TRPL traces are strongly peaked on a short time scale which can not be resolved by measurements due to a limited detector time resolution. Thus, to obtain good agreement with the experimentally recorded Purcell-enhanced TRPL traces a convolution with the Gaussian detector-response function (choosing the FWHM equal to the detectors time resolution) is performed (solid lines).

The direct comparison between measured and calculated TRPL traces is particularly important to confirm that the light-matter coupling in the microscopic model is chosen correctly. We point out that this is non-trivial for gain media with continuous density of states, as there is not a single parameter that can be cast into the form of a spontaneous-emission rate. Instead, contributions from carriers carrying different momenta in the vicinity of the cavity-mode energy contribute together. The agreement of the numerically calculated TRPL traces and the experiment are, therefore, highly valuable and confirm the adequateness of the theoretical description.

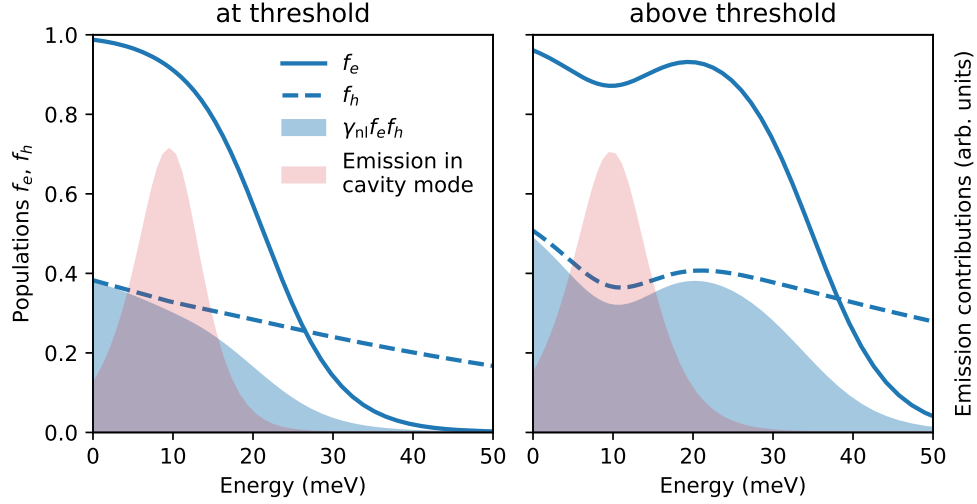

FIG. S6. As a function of energy, we illustrate the influence of the carrier population functions for electrons ( $f_e$ ) and holes ( $f_h$ ) on the SE rate. At the threshold (left panel), the population functions still resemble the thermal case. Above the threshold (right panel), this is no longer the case, as hole burning clamps electron and hole populations in the vicinity of the cavity-mode energy shown in red. Increasing the excitation power results in the population of energetically higher states in the band structure, which increases the overall SE losses into nonlasing modes (indicated in blue), thereby lowering  $\beta$ .

#### Excitation power dependent $\beta$ factor

The  $\beta$  factor plays a fundamental role in rate-equation analysis where it generally is presented as a constant parameter. Here, instead, we model interacting, dynamical subsystems on a microscopic level, and the determining parameters are the light-matter coupling constant  $g_k$  that represents the emission into the laser mode, and the radiative loss rate  $\gamma_{nl}$ . While the  $\beta$  factor does not enter the theory as an input parameter, it can still be expressed as the ratio of the spontaneous emission into the lasing mode over the emission into all modes and can be calculated as such. Specifically,

$$\beta = \frac{\sum_k \frac{2|g_k|^2}{\Gamma + \kappa} L(k) f_k^e f_k^h}{\sum_k \left( \frac{2|g_k|^2}{\Gamma + \kappa} L(k) + \gamma_{nl} \right) f_k^e f_k^h}, \quad (\text{S24})$$

which is derived by adiabatically solving Eq. (S10) and inserting it into Eq. (S7) using Eq. (S16) as the lineshape function  $L(k)$ .

The appearance of the population functions in the above equation lead to an excitation-power dependence of  $\beta$ , as shown in Fig. 3 (c,d). It reaches its maximum just before stimulated emission in the system sets in at an intracavity photon number  $\langle b^\dagger b \rangle \approx 1$ . The subsequent reduction of  $\beta$  is due to population clamping of  $k$  states at the cavity-mode resonance, while other states still experience an increase in population increasing radiative losses into other modes.

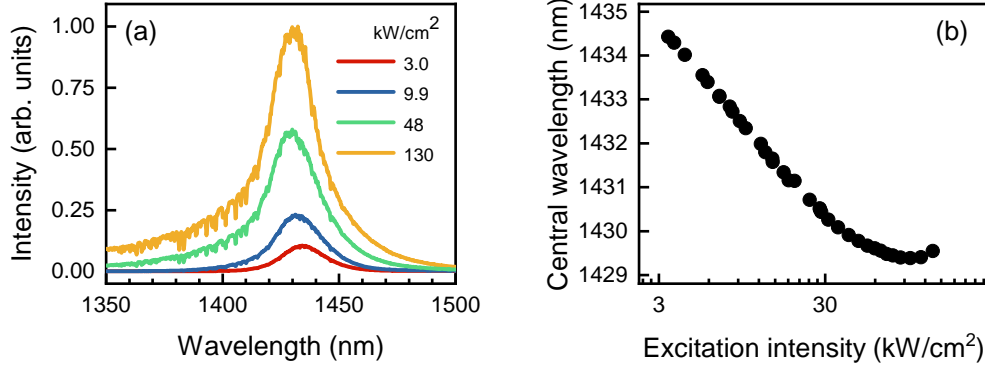

FIG. S7. (a) Exemplary spectra of the emission from the planar material at the excitation intensities noted in the figure at  $T = 10$  K. (b) The extracted central wavelength of the gain spectra with respect to the excitation intensity. The slight distortions measured in (a) are caused by absorption in humid air (in the detection path).

To better illustrate the origin of this effect, we compare the quasi-equilibrium case that is often considered to the microscopic model used here. In quasi-equilibrium, clamping of the total carrier density sets in at the laser threshold, an effect which refers to the total carrier density remaining constant, while excess pump power is converted into emitted photons. In a microscopic picture, one can see that the carrier populations may still increase in parts of the band structure that are not depleted by stimulated emission into the laser mode. As a consequence, the carrier distribution functions become non-thermal and exhibit hole-burning around the cavity resonance, as illustrated in Fig. S6. This decrease of  $\beta$  is a result of this effect: The SE rate in the laser mode no longer increases, as the populations around the cavity mode (indicated in red) are fixed by the hole-burning effect. With increasing pumping, carriers accumulate in higher-lying  $k$  states, which in effect increases radiative losses into non-lasing modes (indicated by the area shaded in blue), thereby lowering  $\beta$ .

Note that other effects have been discussed in the past to modify the SE rate and to lead to a non-constant  $\beta$ , such as line-shape effects, spectral detuning, and dephasing [8–10]. In [11], account has been given to relate the optical and electronic density of states to the SE rate and  $\beta$  in QD-wetting-layer cavity-QED systems. Also in QD systems, sub- and superradiant modifications of the SE rate have also been demonstrated to cause excitation-regime dependent changes of  $\beta$  [12].

We would like to mention that, in principle, also an excitation power dependent spectral detuning between the gain spectrum and the laser mode could influence the  $\beta$ -factor. To shine more light on that, we measured the excitation power dependent gain spectrum and compare the power dependent spectral shift of the gain maximum with that of the laser modes as presented in Fig. 3 e, f. The data was recorded in a planar area of the sample material because it was not possible to follow power dependence of the gain spectrum along with the laser mode of an CNL due to the dominating role of the latter at elevated excitation powers. Further work could address the joint power dependence of the gain spectrum and the laser mode in more favorable cavity geometries, such as micropillar cavities which allow for simultaneous access to the gain spectrum and the laser mode via a  $90^\circ$  axial/lateral detection scheme [13, 14]. The same configuration can also provide experimental access to explore the excitation-power dependence of  $\beta$  for micropillar lasers by comparing emission into non-lasing modes via lateral detection and emission into the lasing mode via axial detection in future work.

In Fig. S7a we show a selection of the measured gain spectra at the different excitation intensities at 10 K. We observe only very modest changes in the measured spectra, when altering the excitation intensity over almost two orders of magnitude. For a quantitative analysis of the power dependent spectra we employ Lorentzian-shaped fit function to extract the optical properties of the emitted light. This lineshape suits well with the measured spectra at low excitation intensities. At higher excitation intensities an asymmetry in the lineshape becomes evident in the short wavelength region. Still, the central wavelengths of the measured spectra can be extracted with good accuracy from the fits, and in Fig. S7b we illustrate that with respect to the growing excitation intensity. The gain that is located near  $1.43 \mu\text{m}$  shows a blue shift of about 5 nm in the relevant power range until a red shift sets in due to heating. Interestingly, the observed spectral shift is almost identical to the power dependent spectral shift of the CNL modes in Fig. 3 e, f. This investigation supports our interpretation of the power dependent  $\beta$ -factor in terms of the excitation power dependent carrier populations, and we can rule out a significant contribution of an excitation power

|                       | CNL1                    | CNL2                    |
|-----------------------|-------------------------|-------------------------|
| $\kappa$              | $0.634 \text{ ps}^{-1}$ | $0.782 \text{ ps}^{-1}$ |
| $\Gamma$              | $5 \text{ ps}^{-1}$     | $5 \text{ ps}^{-1}$     |
| $\gamma_{\text{rel}}$ | $10 \text{ ps}^{-1}$    | $10 \text{ ps}^{-1}$    |
| $g_0$                 | $0.4 \text{ ps}^{-1}$   | $0.38 \text{ ps}^{-1}$  |
| $A$                   | $0.036 \mu\text{m}^2$   | $0.04 \mu\text{m}^2$    |
| $\gamma_{\text{nl}}$  | $0.003 \text{ ps}^{-1}$ | $0.2 \text{ ps}^{-1}$   |

TABLE S1. Summary of explicit parameter values as used for modeling the CNL1 and CNL2.

dependent spectral detuning of the spectral detuning between the gain spectrum and the laser mode on the  $\beta$ -factor.

### Discussion of model parameters

From FDTD calculations cavity  $Q$ -factor and wavelength  $\lambda$ , both relating to the cavity decay rate  $\kappa = \frac{\pi c}{Q\lambda}$ , were determined for both devices CNL1 and CNL2. In both cases, the relaxation rate was assumed to be  $\gamma_{\text{rel}} = 10 \text{ ps}^{-1}$  and the dephasing  $\Gamma = 5 \text{ ps}^{-1}$ , which corresponds to typical values in semiconductor QWs [2]. In the present case of high- $\beta$  lasing we have a strong light-matter interaction due to electric fields strongly confined to dimensions of the light wavelength as well as carrier confinement to the QW plain. Thus, we expect fast radiative recombination into the lasing mode. However, a prerequisite for the successful application of the cluster expansion technique is the absence of strong coupling of the light-matter interaction as defined in cavity QED [3]. That we are indeed in the regime of weak coupling can be seen when adiabatically solving Eq. (S10) while inserting the resulting expressions in the remaining equations of motion. Doing so reveals that for the most strongly coupled  $k$  states, i.e. those resonant with the cavity mode, the ratio of coupling strength to damping in the system is given by

$$C = \frac{2|g_k|^2}{\kappa + \Gamma}.$$

In the present case we have  $C < 0.03$ , asserting the claim to be in the weak coupling regime. In comparison to QD lasers, where the value for the light-matter interaction can be directly determined from time resolved luminescence measurements [3], this is not feasible in the present case. However, we fix the value of  $g_{k=0}$  (see Eqs. (S5)–(S6)) by reproducing the experimentally recorded time resolved luminescence of the CNLs as discussed above.

In the quantum theory of light-matter interaction between a spatially homogeneous light field and the carriers in a QW (as encountered in VCSELs), one normally considers Bloch waves as electronic basis states in the QW with in-plane momenta  $\mathbf{k}_{\parallel}$  [15]

$$\varphi_{\mathbf{k}_{\parallel}}(\mathbf{r}) = \frac{1}{A} e^{-i\mathbf{k}_{\parallel} \cdot \mathbf{r}_{\parallel}} \xi(z) \mathbf{u}_{\mathbf{k}_{\parallel}}(r), \quad (\text{S25})$$

where  $A$  is the quantization area that arises in the standard treatment of QW electronic states in the Bloch formalism. For homogeneous systems, this area is canceled in the transition to a quasi continuum of states. Here, however, the encountered situation is somewhat different. The strong localization of the mode breaks the translation invariance of the system and forces it to choose a quantization area in the limit of a quasi continuum, which we use to evaluate the sums in Eqs. (S7) and (S12). At the same time the strong electric fields in the localized cavity mode lead to a range of local effects, like spatial hole burning and spatially varying interaction strength. As a consequence, and since including the mentioned effects is beyond the scope of our model, we treat the quantization area as an effective parameter. It can be thought of as a measure for the amount of charge carriers that interact with the cavity mode, which is similar to the number of quantum dots, each containing one exciton, in a quantum-dot-based nanolaser [3, 5]. The areas used in the modeling of CNL1 to CNL2 reflect the relative size of the QW structures as well as their relative overlap with the cavity mode. The parameters used in modeling of the CNLs are discussed above and their explicit values are summarized in Table S1 for better overview.

- 
- [1] Khajavikhan, M. *et al.* Thresholdless nanoscale coaxial lasers. *Nature* **482**, 204–207 (2012).
  - [2] Chow, W. W. & Koch, S. W. *Semiconductor-Laser Fundamentals: Physics of the Gain Materials* (Springer-Verlag, Berlin Heidelberg, 1999).
  - [3] Gies, C., Wiersig, J., Lorke, M. & Jahnke, F. Semiconductor model for quantum-dot-based microcavity lasers. *Phys. Rev. A* **75**, 013803 (2007).
  - [4] Chow, W. W., Crawford, M. H., Tsao, J. Y. & Kneissl, M. Internal efficiency of InGaN light-emitting diodes: Beyond a quasiequilibrium model. *Appl. Phys. Lett.* **97**, 121105 (2010).
  - [5] Lohof, F., Barzel, R., Gartner, P. & Gies, C. Delayed transition to coherent emission in nanolasers with extended gain media. *Phys. Rev. Appl.* **10**, 054055 (2018).
  - [6] Ates, S. *et al.* Influence of the spontaneous optical emission factor  $\beta$  on the first-order coherence of a semiconductor microcavity laser. *Phys. Rev. B* **78**, 155319 (2008).
  - [7] Loudon, R. *The Quantum Theory of Light* (Oxford University Press, Oxford, New York, 2000), third edition edn.
  - [8] Fujita, M., Ushigome, R. & Baba, T. Large spontaneous emission factor of 0.1 in a microdisk injection laser. *Photon. Technol. Lett.* **13**, 403 (2001).
  - [9] Englund, D. *et al.* Controlling the spontaneous emission rate of single quantum dots in a two-dimensional photonic crystal. *Phys. Rev. Lett.* **95**, 013904 (2005).
  - [10] Sumikura, H., Kuramochi, E., Taniyama, H. & Notomi, M. Purcell enhancement of fast-dephasing spontaneous emission from electron-hole droplets in high- $q$  silicon photonic crystal nanocavities. *Phys. Rev. B* **94**, 195314 (2016).
  - [11] Gregersen, N., Suhr, T., Lorke, M. & Mørk, J. Quantum-dot nano-cavity lasers with Purcell-enhanced stimulated emission. *Appl. Phys. Lett.* **100**, 131107 (2012).
  - [12] Lichtmannecker, S. *et al.* A few-emitter solid-state multi-exciton laser. *Sci. Rep.* **7**, 7420 (2017).
  - [13] Musiał, A. *et al.* Correlations between axial and lateral emission of coupled quantum dot–micropillar cavities. *Phys. Rev. B* **91**, 205310 (2015). URL <https://link.aps.org/doi/10.1103/PhysRevB.91.205310>.
  - [14] Holzinger, S. *et al.* Determining the linewidth enhancement factor via optical feedback in quantum dot micropillar lasers. *Opt. Express* **26**, 31363–31371 (2018).
  - [15] Kira, M., Jahnke, F., Hoyer, W. & Koch, S. W. Quantum theory of spontaneous emission and coherent effects in semiconductor microstructures. *Prog. Quantum. Electron.* **23**, 189–279 (1999).
